# Supplementary material for: HyperFormer: Enhancing Entity and Relation Interaction for Hyper-Relational Knowledge Graph Completion
Source: arXiv:2308.06512 source file (2023-08-12)
Supplement: Supplementary file 1 [file appendix.tex]

\subsection*{A Details about Experiments}
In this section, we give more experimental details, mainly including hyper-parameter settings, the statistics of different datasets, and the evaluation protocol.

\paragraph{Hyper-parameter Settings.} Table~\ref{table_hyperparameters} shows the main hyperparameter settings of HyperFormer  on the WD50K, WikiPeople, and JF17K datasets. All experiments are conducted on a 32G Tesla V100 GPU, and implemented our method with PyTorch. We employ  AdamW as the optimizer and a cosine decay scheduler with linear warm-up is used for optimization. All hyperparameters are tuned according to the MRR metric on the validation set.

\begin{table}[!hp]

\setlength{\tabcolsep}{0.30em}
\centering
\small
\begin{tabular*}{\linewidth}{@{}cc@{}}
\toprule
\multicolumn{1}{l}{\textbf{Parameter}} & \multicolumn{1}{c}{\textbf{\{WD50K,\,\, WikiPeople,\,\, JF17K\}}} \\
\midrule
\multicolumn{1}{l}{\# Epochs}   &\multicolumn{1}{c}{\{100,\,\,\,100,\,\,\,100\}} \\
\multicolumn{1}{l}{\# Batch size}   &\multicolumn{1}{c}{\{256,\,\,\,256,\,\,\,256\}} \\
\multicolumn{1}{l}{\# Entity neighbor}   &\multicolumn{1}{c}{\{3,\,\,\,3,\,\,\,3\}} \\
\multicolumn{1}{l}{\# Qualifiers neighbor}   &\multicolumn{1}{c}{\{6,\,\,\,6,\,\,\,6\}} \\
\multicolumn{1}{l}{\# Learning rate}   &\multicolumn{1}{c}{\{0.0006,\,\,\,0.0006,\,\,\,0.0006\}} \\
\multicolumn{1}{l}{\# Label smoothing}   &\multicolumn{1}{c}{\{0.9,\,\,\,0.9,\,\,\,0.9\}} \\
\multicolumn{1}{l}{\# Trm layers}   &\multicolumn{1}{c}{\{8,\,\,\,8,\,\,\,8\}} \\
\multicolumn{1}{l}{\# Trm hidden dim}   &\multicolumn{1}{c}{\{400,\,\,\,400,\,\,\,400\}} \\
\multicolumn{1}{l}{\# Trm heads}   &\multicolumn{1}{c}{\{2,\,\,\,2,\,\,\,2\}} \\
\multicolumn{1}{l}{\# Trm input dropout}   &\multicolumn{1}{c}{\{0.7,\,\,\,0.7,\,\,\,0.7\}} \\
\multicolumn{1}{l}{\# Trm hidden dropout}   &\multicolumn{1}{c}{\{0.1,\,\,\,0.1,\,\,\,0.1\}} \\
\multicolumn{1}{l}{\# Conv input dropout}   &\multicolumn{1}{c}{\{0.2,\,\,\,0.2,\,\,\,0.2\}} \\
\multicolumn{1}{l}{\# Conv hidden dropout}   &\multicolumn{1}{c}{\{0.5,\,\,\,0.5,\,\,\,0.5\}} \\
\multicolumn{1}{l}{\# Conv channel}   &\multicolumn{1}{c}{\{96,\,\,\,96,\,\,\,96\}} \\
\multicolumn{1}{l}{\# Conv kernel size}   &\multicolumn{1}{c}{\{9,\,\,\,9,\,\,\,9\}} \\
\multicolumn{1}{l}{\# MoE experts}   &\multicolumn{1}{c}{\{64,\,\,\,64,\,\,\,64\}} \\
\multicolumn{1}{l}{\# MoE top experts}   &\multicolumn{1}{c}{\{2,\,\,\,2,\,\,\,2\}} \\
\bottomrule
\end{tabular*}
\caption{The main hyperparameters of Hy[erFormer] model in different datasets. Trm, Conv, and MoE are the abbreviations of Transformer, Convolution, and Mixture-of-Experts, respectively.}
\label{table_hyperparameters}
\end{table}

\paragraph{Datasets.}
We conducted experiments on three well-known datasets, WD50K~\citep{Mikhail_2020}, WikiPeople~\citep{Saiping_2019}, and JF17K~\citep{Jianfeng_2016}. In order to explore the effectiveness of HyperFormer under different ratio of  qualifier pairs, and with different number of neighbors, we further constructed two datasets, see Section~\ref{section_datasets_and_baselines}. All datasets statistics are presented in Table~\ref{table_statistics_datasets}. 

%For each dataset, we construct three subsets, corresponding to 33\%, 66\%, and 100\% of  facts with hyper-relational knowledge. To evaluate the performance difference of the models on different degrees of entities, we use the dataset containing 100\% hyper-relational as the basic data, for the training set, construct subsets in which the corresponding entity contains only from one to foure neighbors, and the validation and test set are kept unchanged. All datasets statistics are presented in Table~\ref{table_statistics_datasets}.

\paragraph{Evaluation Protocol.}
We evaluate the model performance using two common metrics: MRR and Hits@\emph{N} (abbreviated as H@\emph{N}). MRR is the average of reciprocal ranking, and Hits@\emph{N} is the proportion of top \emph{N}, we select \emph{N}=\{1,3,10\}. The larger value of both metrics, the better the effect of the corresponding model.

\subsection*{B Additional Results}
\begin{enumerate}[itemsep=0.5ex, leftmargin=5mm]
\item Table~\ref{table_different_hyper_ratio_result_wd50k} shows  detailed results on the WD50K dataset with different ratio of qualifiers.
\item Table~\ref{table_different_hyper_ratio_result_wikipeople} shows  detailed results on the WikiPeople dataset with different ratio of qualifiers.
\item Table~\ref{table_different_hyper_ratio_result_jf17k} shows  detailed results on the JF17K dataset with different ratio of qualifiers.
\item Table~\ref{table_different_degree_wd50k_100} shows  detailed results on the WD50K dataset with different degrees of entity.
\item Table~\ref{table_different_degree_wikipeople_100} shows  detailed results on the WikiPeople dataset with different degrees of entity.
\item Table~\ref{table_different_degree_jf17k_100} shows  detailed results on the JF17K dataset with different degrees of entity.
\item Table~\ref{table_different_translation_methods} shows  detailed results of selecting different transaction methods to compose the qualifier entity and qualifier relation. Specifically, we adopt four transaction methods, i.e., TransE~\citep{Antoine_2013}, DistMult~\citep{Bishan_2015}, ComplEx~\citep{TrouillonWRGB_2016}, and RotatE~\citep{Zhiqing_2019}.
\end{enumerate}

\begin{table*}[!htp]

\setlength{\tabcolsep}{0.58em}
\centering
\small
\begin{tabular*}{0.95\linewidth}{@{}ccccccccc@{}}
\hline
\multicolumn{1}{c}{\textbf{Datasets}} &\multicolumn{1}{c}{\textbf{w/ Quals(\%)}} &\multicolumn{1}{c}{\textbf{Train}} &\multicolumn{1}{c}{\textbf{Valid}} &\multicolumn{1}{c}{\textbf{Test}} &\multicolumn{1}{c}{\textbf{Entity}} &\multicolumn{1}{c}{\textbf{Relation}} &\multicolumn{1}{c}{\textbf{E in quals}} &\multicolumn{1}{c}{\textbf{R in quals}}\\
\hline
WD50K   &32167(13.6\%)  &166435  &23913  &46159  &47155  &531  &5459  &44 \\
WD50K (33)   &31866(31.2\%)  &73406  &10568  &18133  &38123  &474  &6466  &46 \\
WD50K (66)  &31696(64.5\%)  &35968  &5154  &8045  &27346  &403  &7212  &52 \\
WD50K (100)  &32167(100\%)  &22738  &3279  &5297  &18791  &278  &7917  &74 \\
WD50K (100) \#1   &10767(100\%)  &2191  &3279  &5297  &10375  &189  &4768  &66 \\
WD50K (100) \#2   &12958(100\%)  &4382  &3279  &5297  &11241  &200  &5340  &66 \\
WD50K (100) \#3   &15123(100\%)  &6547  &3279  &5297  &11985  &207  &5818  &67 \\
WD50K (100) \#4   &17082(100\%)  &8506  &3279  &5297  &12649  &210  &6226  &67 \\
\hline
WikiPeople   &9482(2.6\%)  &294439  &37715  &37712  &34825  &178  &415  &34 \\
WikiPeople (33)   &11673(33\%)  &28280  &3550  &3542  &20921  &145  &803  &40 \\
WikiPeople (66)  &11673(66\%)  &14130  &1782  &1774  &13651  &133  &1076  &47 \\
WikiPeople (100)  &11673(100\%)  &9319  &1181  &1173  &8068  &105  &1310  &57 \\
WikiPeople (100) \#1   &2607(100\%)  &1253  &1181  &1173  &4212  &83  &799  &48 \\
WikiPeople (100) \#2   &4852(100\%)  &2498  &1181  &1173  &4711  &85  &948  &50 \\
WikiPeople (100) \#3   &6001(100\%)  &3647  &1181  &1173  &5040  &87  &1017  &51 \\
WikiPeople (100) \#4   &6869(100\%)  &4515  &1181  &1173  &5338  &89  &1088  &52 \\
\hline
JF17K   &46320(45.9\%)  &76379  &-  &24568  &28645  &501  &3651  &179 \\
JF17K (33)   &24484(33\%)  &56959  &8122  &9112  &24081  &490  &2331  &173 \\
JF17K (66)  &24484(66\%)  &27280  &4413  &5403  &19288  &469  &3094  &173 \\
JF17K (100)  &24484(100\%)  &17190  &3152  &4142  &12656  &307  &3648  &173 \\
JF17K (100) \#1   &9786(100\%)  &2492  &3152  &4142  &7320  &253  &1846  &142 \\
JF17K (100) \#2   &12278(100\%)  &4984  &3152  &4142  &7930  &255  &2212  &143 \\
JF17K (100) \#3   &14588(100\%)  &7294  &3152  &4142  &8367  &257  &2424  &144 \\
JF17K (100) \#4   &16513(100\%)  &9219  &3152  &4142  &8688  &259  &2556  &145 \\
\bottomrule
\end{tabular*}
\caption{Statistics of datasets. E in quals (R in quals) denote the amount of entities (relations) appearing only in qualifier pairs. The values in parentheses indicate that the corresponding percentage in corresponding dataset has hyper-relational facts. The value behind \# indicates that the entity in the training set only contains the number of neighbors with the corresponding value. }
\label{table_statistics_datasets}
\end{table*}

\begin{table*}[!htp]

\setlength{\tabcolsep}{0.24em}
\centering
\small
\begin{tabular*}{\linewidth}{@{}ccccccccccccc@{}}
\hline
\multicolumn{1}{c}{\multirow{2}{*}{\textbf{Methods}}} & \multicolumn{4}{c}{\textbf{WD50K (33)}} & \multicolumn{4}{c}{\textbf{WD50K (66)}} & \multicolumn{4}{c}{\textbf{WD50K (100)}}\\
\cmidrule(lr){2-5}\cmidrule(lr){6-9}\cmidrule(l){10-13}
& \textbf{MRR} & \textbf{H@1} & \textbf{H@3}   & \textbf{H@10} & \textbf{MRR} & \textbf{H@1} & \textbf{H@3} & \textbf{H@10} & \textbf{MRR}  & \textbf{H@1} & \textbf{H@3} & \textbf{H@10} \\
\hline
StarE~\citep{Mikhail_2020}   &0.308  &0.247  &0.335  &0.423  &0.449  &0.388  &0.480  &0.566    &0.610  &0.543  &0.649  &0.734 \\
Hy-Transformer~\citep{Donghan_2021}   &0.313  &0.255  &0.337  &0.425  &0.458  &0.397  &0.491  &0.574    &0.621  &0.557  &0.659  &0.738 \\
GRAN~\citep{Quan_2021}   &0.322  &0.269  &0.344  &0.425  &0.472  &0.419  &0.500  &0.573    &0.647  &0.593  &0.677  &0.747 \\
QUAD~\citep{Harry_2022}   &0.329  &0.266  &0.357  &0.447  &0.479  &0.416  &0.513  &0.593    &0.646  &0.572  &0.691  &\textbf{0.778} \\
HyperFormer   &\textbf{0.338}  &\textbf{0.280}  &\textbf{0.362}  &\textbf{0.450}  &\textbf{0.492}  &\textbf{0.434}  &\textbf{0.523}  &\textbf{0.597}    &\textbf{0.666}  &\textbf{0.611}  &\textbf{0.698}  &0.770 \\
\bottomrule
\end{tabular*}
\caption{Evaluation of different models on WD50K with different ratio of qualifiers. Best scores are highlighted in \textbf{bold}.}
\label{table_different_hyper_ratio_result_wd50k}
\end{table*}

\begin{table*}[!htp]

\setlength{\tabcolsep}{0.23em}
\centering
\small
\begin{tabular*}{\linewidth}{@{}ccccccccccccc@{}}
\hline
\multicolumn{1}{c}{\multirow{2}{*}{\textbf{Methods}}} & \multicolumn{4}{c}{\textbf{WikiPeople (33)}} & \multicolumn{4}{c}{\textbf{WikiPeople (66)}} & \multicolumn{4}{c}{\textbf{WikiPeople (100)}}\\
\cmidrule(lr){2-5}\cmidrule(lr){6-9}\cmidrule(l){10-13}
& \textbf{MRR} & \textbf{H@1} & \textbf{H@3}   & \textbf{H@10} & \textbf{MRR} & \textbf{H@1} & \textbf{H@3} & \textbf{H@10} & \textbf{MRR}  & \textbf{H@1} & \textbf{H@3} & \textbf{H@10} \\
\hline
StarE~\citep{Mikhail_2020}   &0.192  &0.143  &0.211  &0.285  &0.259  &0.205  &0.284  &0.360    &0.343  &0.279  &0.374  &0.465 \\
Hy-Transformer~\citep{Donghan_2021}   &0.192  &0.140  &0.209  &0.297  &0.268  &0.215  &0.297  &0.367    &0.372  &0.316  &0.401  &0.478 \\
GRAN~\citep{Quan_2021}   &0.201  &0.156  &0.220  &0.284  &0.287  &0.244  &0.310  &0.359    &0.403  &0.349  &0.437  &0.490 \\
QUAD~\citep{Harry_2022}   &0.204  &0.155  &0.224  &0.297  &0.282  &0.228  &0.315  &0.373    &0.385  &0.318  &0.430  &0.497 \\
HyperFormer   &\textbf{0.213}  &\textbf{0.161}  &\textbf{0.232}  &\textbf{0.312}  &\textbf{0.298}  &\textbf{0.255}  &\textbf{0.316}  &\textbf{0.376}    &\textbf{0.426}  &\textbf{0.373}  &\textbf{0.454}  &\textbf{0.527} \\
\bottomrule
\end{tabular*}
\caption{Evaluation of different models on WikiPeople with different ratio of qualifiers. Best scores are highlighted in \textbf{bold}.}
\label{table_different_hyper_ratio_result_wikipeople}
\end{table*}

\begin{table*}[!htp]

\setlength{\tabcolsep}{0.23em}
\centering
\small
\begin{tabular*}{\linewidth}{@{}ccccccccccccc@{}}
\hline
\multicolumn{1}{c}{\multirow{2}{*}{\textbf{Methods}}} & \multicolumn{4}{c}{\textbf{JF17K (33)}} & \multicolumn{4}{c}{\textbf{JF17K (66)}} & \multicolumn{4}{c}{\textbf{JF17K (100)}}\\
\cmidrule(lr){2-5}\cmidrule(lr){6-9}\cmidrule(l){10-13}
& \textbf{MRR} & \textbf{H@1} & \textbf{H@3}   & \textbf{H@10} & \textbf{MRR} & \textbf{H@1} & \textbf{H@3} & \textbf{H@10} & \textbf{MRR}  & \textbf{H@1} & \textbf{H@3} & \textbf{H@10} \\
\hline
StarE~\citep{Mikhail_2020}   &0.290  &0.197  &0.320  &0.484  &0.302  &0.214  &0.340  &0.478    &0.321  &0.223  &0.366  &0.519 \\
Hy-Transformer~\citep{Donghan_2021}   &0.298  &0.204  &0.333  &0.493  &0.325  &0.234  &0.365  &0.510    &0.361  &0.266  &0.407  &0.542 \\
GRAN~\citep{Quan_2021}   &0.307  &0.212  &0.342  &0.498  &0.326  &0.237  &0.367  &0.500    &0.382  &0.290  &0.429  &0.567 \\
QUAD~\citep{Harry_2022}   &0.307  &0.210  &0.344  &0.504  &0.334  &0.241  &0.374  &0.520    &0.379  &0.277  &0.430  &0.581 \\
HyperFormer   &\textbf{0.352}  &\textbf{0.254}  &\textbf{0.391}  &\textbf{0.545}  &\textbf{0.411}  &\textbf{0.325}  &\textbf{0.446}  &\textbf{0.598}    &\textbf{0.478}  &\textbf{0.396}  &\textbf{0.515}  &\textbf{0.645} \\
\bottomrule
\end{tabular*}
\caption{Evaluation of different models on JF17K with different ratio of qualifiers. Best scores are highlighted in \textbf{bold}.}
\label{table_different_hyper_ratio_result_jf17k}
\end{table*}

\begin{table*}[!htp]

\setlength{\tabcolsep}{0.21em}
\centering
\small
\begin{tabular*}{\linewidth}{@{}ccccccccccccc@{}}
\hline
\multicolumn{1}{c}{\multirow{2}{*}{\textbf{Methods}}} & \multicolumn{3}{c}{\textbf{WD50K (100) \#1}} & \multicolumn{3}{c}{\textbf{WD50K (100) \#2}} & \multicolumn{3}{c}{\textbf{WD50K (100) \#3}} & \multicolumn{3}{c}{\textbf{WD50K (100) \#4}}\\
\cmidrule(lr){2-4}\cmidrule(lr){5-7}\cmidrule(lr){8-10}\cmidrule(l){11-13}
& \textbf{MRR} & \textbf{H@1}   & \textbf{H@10} & \textbf{MRR} & \textbf{H@1} & \textbf{H@10} & \textbf{MRR}  & \textbf{H@1} & \textbf{H@10} & \textbf{MRR} & \textbf{H@1} & \textbf{H@10}\\
\hline
StarE~\citep{Mikhail_2020}   &0.104  &0.056  &0.203  &0.208  &0.143  &0.343  &0.313  &0.242    &0.456  &0.369  &0.300  &0.504 \\
Hy-Transformer~\citep{Donghan_2021}   &0.071  &0.032  &0.161  &0.167  &0.097  &0.322  &0.315  &0.250    &0.446  &0.374  &0.311  &0.499 \\
GRAN~\citep{Quan_2021}   &0.125  &0.088  &0.195  &0.235  &0.184  &0.333  &0.327  &0.269    &0.441  &0.374  &0.317  &0.484 \\
QUAD~\citep{Harry_2022}   &0.065  &0.022  &0.161  &0.134  &0.062  &0.285  &0.284  &0.197    &0.463  &0.371  &0.286  &\textbf{0.529} \\
HyperFormer   &\textbf{0.193}  &\textbf{0.140}  &\textbf{0.302}  &\textbf{0.303}  &\textbf{0.242}  &\textbf{0.422}  &\textbf{0.374}  &\textbf{0.305}    &\textbf{0.510}  &\textbf{0.410}  &\textbf{0.352}  &\textbf{0.529} \\
\bottomrule
\end{tabular*}
\caption{Evaluation of different models on WD50K (100) with different degrees of entity. Best scores are highlighted in \textbf{bold}.}
\label{table_different_degree_wd50k_100}
\end{table*}

\begin{table*}[!htp]

\setlength{\tabcolsep}{0.19em}
\centering
\small
\begin{tabular*}{\linewidth}{@{}ccccccccccccc@{}}
\hline
\multicolumn{1}{c}{\multirow{2}{*}{\textbf{Methods}}} & \multicolumn{3}{c}{\textbf{WikiPeople (100) \#1}} & \multicolumn{3}{c}{\textbf{WikiPeople (100) \#2}} & \multicolumn{3}{c}{\textbf{WikiPeople (100) \#3}} & \multicolumn{3}{c}{\textbf{WikiPeople (100) \#4}}\\
\cmidrule(lr){2-4}\cmidrule(lr){5-7}\cmidrule(lr){8-10}\cmidrule(l){11-13}
& \textbf{MRR} & \textbf{H@1}   & \textbf{H@10} & \textbf{MRR} & \textbf{H@1} & \textbf{H@10} & \textbf{MRR}  & \textbf{H@1} & \textbf{H@10} & \textbf{MRR} & \textbf{H@1} & \textbf{H@10}\\
\hline
StarE~\citep{Mikhail_2020}   &0.121  &0.077  &0.203  &0.112  &0.071  &0.194  &0.193  &0.127    &0.339  &0.255  &0.191  &0.371 \\
Hy-Transformer~\citep{Donghan_2021}   &0.091  &0.061  &0.150  &0.148  &0.098  &0.245  &0.186  &0.133    &0.282  &0.233  &0.169  &0.351 \\
GRAN~\citep{Quan_2021}    &0.119  &0.087  &0.174  &0.186  &0.142  &0.263  &0.242  &0.190    &0.336  &0.273  &0.220  &0.377 \\
QUAD~\citep{Harry_2022}    &0.075  &0.053  &0.120  &0.140  &0.088  &0.231  &0.186  &0.121    &0.318  &0.255  &0.190  &0.384 \\
HyperFormer   &\textbf{0.194}  &\textbf{0.148}  &\textbf{0.283}  &\textbf{0.252}  &\textbf{0.209}  &\textbf{0.335}  &\textbf{0.303}  &\textbf{0.255}    &\textbf{0.395}  &\textbf{0.328}  &\textbf{0.283}  &\textbf{0.414} \\
\bottomrule
\end{tabular*}
\caption{Evaluation of different models on WikiPeople (100) with different degrees of entity. Best scores are highlighted in \textbf{bold}.}
\label{table_different_degree_wikipeople_100}
\end{table*}

\begin{table*}[!htp]

\setlength{\tabcolsep}{0.21em}
\centering
\small
\begin{tabular*}{\linewidth}{@{}ccccccccccccc@{}}
\hline
\multicolumn{1}{c}{\multirow{2}{*}{\textbf{Methods}}} & \multicolumn{3}{c}{\textbf{JF17K (100) \#1}} & \multicolumn{3}{c}{\textbf{JF17K (100) \#2}} & \multicolumn{3}{c}{\textbf{JF17K (100) \#3}} & \multicolumn{3}{c}{\textbf{JF17K (100) \#4}}\\
\cmidrule(lr){2-4}\cmidrule(lr){5-7}\cmidrule(lr){8-10}\cmidrule(l){11-13}
& \textbf{MRR} & \textbf{H@1}   & \textbf{H@10} & \textbf{MRR} & \textbf{H@1} & \textbf{H@10} & \textbf{MRR}  & \textbf{H@1} & \textbf{H@10} & \textbf{MRR} & \textbf{H@1} & \textbf{H@10}\\
\hline
StarE~\citep{Mikhail_2020}   &0.169  &0.089  &0.315  &0.249  &0.156  &0.405  &0.275  &0.178    &0.456  &0.286  &0.187  &0.478 \\
Hy-Transformer~\citep{Donghan_2021}   &0.137  &0.085  &0.217  &0.241  &0.148  &0.400  &0.299  &0.195    &0.465  &0.318  &0.212  &0.499 \\
GRAN~\citep{Quan_2021}    &0.203  &0.121  &0.352  &0.267  &0.169  &0.449  &0.284  &0.185    &0.474  &0.301  &0.200  &0.496 \\
QUAD~\citep{Harry_2022}    &0.228  &0.138  &0.385  &0.241  &0.141  &0.428  &0.280  &0.178    &0.471  &0.306  &0.200  &0.499 \\
HyperFormer   &\textbf{0.305}  &\textbf{0.216}  &\textbf{0.453}  &\textbf{0.338}  &\textbf{0.248}  &\textbf{0.492}  &\textbf{0.350}  &\textbf{0.256}    &\textbf{0.515}  &\textbf{0.374}  &\textbf{0.277}  &\textbf{0.553} \\
\bottomrule
\end{tabular*}
\caption{Evaluation of different models on JF17K (100) with different degrees of entity. Best scores are highlighted in \textbf{bold}.}
\label{table_different_degree_jf17k_100}
\end{table*}

\begin{table*}[!htp]

\setlength{\tabcolsep}{0.42em}
\centering
\small
\begin{tabular*}{\linewidth}{@{}ccccccccccccc@{}}
\hline
\multicolumn{1}{c}{\multirow{2}{*}{\textbf{Methods}}} & \multicolumn{4}{c}{\textbf{WD50K (100)}} & \multicolumn{4}{c}{\textbf{WikiPeople (100)}} & \multicolumn{4}{c}{\textbf{JF17K (100)}}\\
\cmidrule(lr){2-5}\cmidrule(lr){6-9}\cmidrule(l){10-13}
& \textbf{MRR} & \textbf{H@1} & \textbf{H@3}   & \textbf{H@10} & \textbf{MRR} & \textbf{H@1} & \textbf{H@3} & \textbf{H@10} & \textbf{MRR}  & \textbf{H@1} & \textbf{H@3} & \textbf{H@10} \\
\hline
HyperFormer-TransE   &0.666  &\textbf{0.611}  &0.697  &0.768  &0.424  &\textbf{0.374}  &0.452  &0.524    &\textbf{0.487}  &\textbf{0.401}  &\textbf{0.526}  &\textbf{0.662} \\
HyperFormer-DistMult   &0.666  &\textbf{0.611}  &\textbf{0.698}  &0.770  &\textbf{0.426}  &0.373  &\textbf{0.454}  &\textbf{0.527}    &0.478  &0.396  &0.515  &0.645 \\
HyperFormer-ComplEx  &\textbf{0.667}  &\textbf{0.611}  &\textbf{0.698}  &0.769  &0.422  &0.370  &0.445  &0.518    &0.479  &0.399  &0.519  &0.642 \\
HyperFormer-RotatE  &0.655  &0.592  &0.690  &\textbf{0.772}  &0.415  &0.371  &0.434  &0.496    &0.479  &\textbf{0.401}  &0.515  &0.644 \\
\bottomrule
\end{tabular*}
\caption{Evaluation of different transaction methods on WD50K(100), WikiPeople(100) and JF17K(100) datasets. Best scores are highlighted in \textbf{bold}.}
\label{table_different_translation_methods}
\end{table*}
